# Supplementary material for: On the detection of internal interfacial layers in turbulent flows
Source: arXiv:1811.09258 source file (2018-11-22)
Supplement: Supplementary file 1 [file JFM2018_Appendix.tex]

\appendix
\section{What is the nature of internal interfacial layers} \label{appA}
\begin{figure}
\centerline{\includegraphics{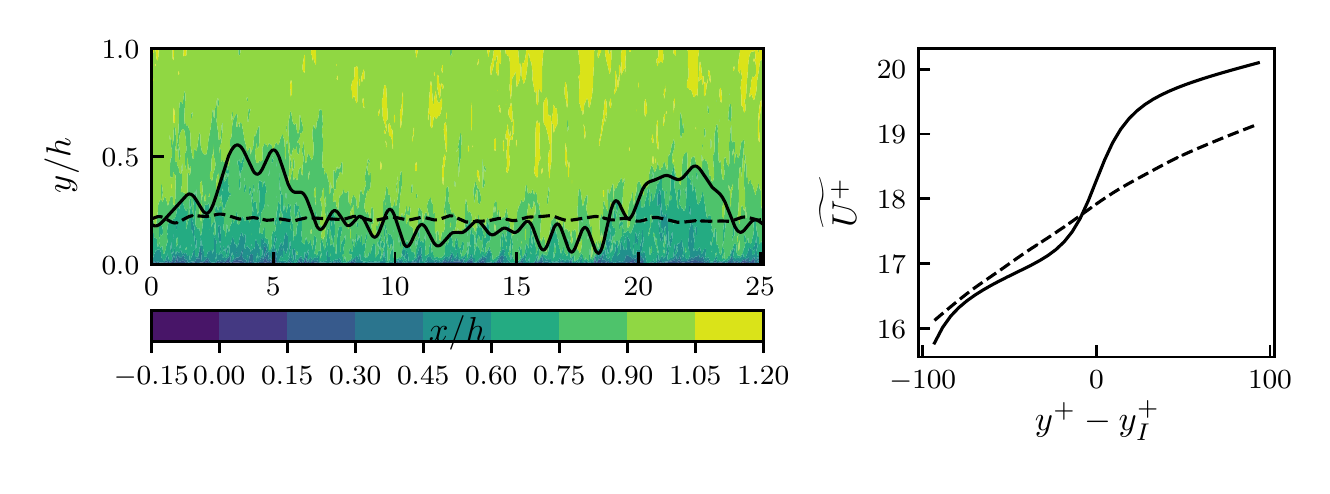}}
\caption{(a)The interfacial layer between Zone 2 and 3 identified from the original velocity field of $Re_{\tau}=950$ channel(solid) and the averaging field with white noise(dashed). (b) The conditional average across IIL in (a) of streamwise velocity}
\label{fig:gaussian}
\end{figure}
\dsf{As highlighted in \citet{meinhart1995existence}, the instantaneous streamwise profile has step-like feature and ILLs exist at where the jump occurs.
The conditional results shown in figure \ref{fig:conditional} give the statistical evidence of their existence. However, the step-like feature relies on
the existence of velocity coherence. If no coherence exists, like velocity field constructed from the mean velocity profile and white noise whose level is
related with the root mean square (R.M.S) velocity profile, the IIL is nearly parallel to the solid wall and have no streak-like feature which is shown in
section \ref{sec:3d}. In addition, the conditional results approaches the conventional average velocity profile(figure \ref{fig:gaussian})(b). 
}
